# Supplementary material for: Character Transformations for Non-Autoregressive GEC Tagging
Source: arXiv:2111.09280 source file (2021-11-17)
Supplement: Supplementary file 1 [file 99_appendix.tex]

\begin{table*}[p]
  \begin{tabular}{@{}llcrrrrrrrrrr@{}} \toprule
    \multirow{2}{*}{Language} & \multirow{2}{*}{Tokenizer} & Min &
      \multicolumn{2}{c}{Word-Whole} & \multicolumn{2}{c}{Subw-Whole} & \multicolumn{2}{c}{Word-Chars} &
      \multicolumn{2}{c}{Subw-Chars} & \multicolumn{2}{c}{Compos} \\ \cmidrule{4-13}
    && Occ & Rules & \multicolumn{1}{c}{F1} & Rules & \multicolumn{1}{c}{F1} & Rules &
      \multicolumn{1}{c}{F1} & Rules & \multicolumn{1}{c}{F1} & Rules & \multicolumn{1}{c}{F1} \\ \midrule
      \multirow{6}{*}{Czech} & \multirow{3}{*}{\shortstack[l]{mBERT\\uncased}} & 3 & 10850 & 63.35 & 8589 & 78.17 & 3767 & 77.58 & 2951 & 87.25 & 1991 & 94.21\\
       &  & 2 & 18536 & 68.39 & 13019 & 81.94 & 7093 & 80.13 & 5143 & 89.03 & 3117 & 94.95\\
       &  & 1 & 41618 & 73.42 & 26854 & 85.67 & 21326 & 83.54 & 15069 & 91.16 & 8638 & 95.84\\
       & \multirow{3}{*}{\shortstack[l]{mBERT\\cased}} & 3 & 5174 & 72.12 & 4169 & 89.03 & 2631 & 83.94 & 2207 & 91.92 & 1852 & 94.37\\
       &  & 2 & 9820 & 76.05 & 6837 & 90.69 & 5098 & 85.54 & 3871 & 93.06 & 2987 & 95.25\\
       &  & 1 & 25911 & 80.60 & 16342 & 92.62 & 16812 & 88.04 & 11669 & 94.38 & 8431 & 96.10\\
      \midrule
      \multirow{9}{*}{English} & \multirow{3}{*}{\shortstack[l]{mBERT\\uncased}} & 3 & 12349 & 86.88 & 12913 & 88.66 & 4527 & 90.83 & 4361 & 92.93 & 4494 & 93.77\\
       &  & 2 & 20292 & 88.64 & 19524 & 90.11 & 7631 & 91.52 & 7359 & 93.38 & 7421 & 94.44\\
       &  & 1 & 53557 & 91.20 & 48383 & 92.25 & 33985 & 93.41 & 32221 & 95.41 & 27371 & 95.85\\
       & \multirow{3}{*}{\shortstack[l]{mBERT\\cased}} & 3 & 7551 & 87.85 & 6979 & 89.86 & 4285 & 90.69 & 4245 & 92.92 & 4448 & 93.85\\
       &  & 2 & 12822 & 89.86 & 10994 & 91.42 & 7275 & 91.41 & 7165 & 93.41 & 7364 & 94.66\\
       &  & 1 & 38440 & 92.05 & 33520 & 93.56 & 33257 & 93.42 & 31485 & 95.49 & 27171 & 96.01\\
       & \multirow{3}{*}{\shortstack[l]{BERT\\cased}} & 3 & 7557 & 88.53 & 6762 & 89.98 & 4283 & 91.87 & 4180 & 93.32 & 4428 & 93.66\\
       &  & 2 & 12805 & 90.08 & 10625 & 91.36 & 7321 & 92.29 & 7092 & 93.65 & 7398 & 94.23\\
       &  & 1 & 38733 & 92.19 & 33209 & 93.26 & 33438 & 93.94 & 31892 & 95.37 & 27564 & 95.77\\
      \midrule
      \multirow{6}{*}{German} & \multirow{3}{*}{\shortstack[l]{mBERT\\uncased}} & 3 & 4577 & 67.04 & 4648 & 72.96 & 1831 & 80.68 & 1673 & 85.23 & 1408 & 91.77\\
       &  & 2 & 7308 & 70.71 & 6863 & 76.40 & 3017 & 82.96 & 2682 & 86.82 & 2110 & 92.74\\
       &  & 1 & 23979 & 76.90 & 18991 & 82.05 & 11676 & 86.01 & 9959 & 89.53 & 6639 & 94.17\\
       & \multirow{3}{*}{\shortstack[l]{mBERT\\cased}} & 3 & 2201 & 75.88 & 2229 & 84.11 & 1608 & 83.47 & 1450 & 89.05 & 1402 & 91.87\\
       &  & 2 & 3754 & 78.91 & 3634 & 86.23 & 2610 & 84.98 & 2340 & 90.07 & 2090 & 92.80\\
       &  & 1 & 14379 & 83.42 & 11844 & 89.14 & 10512 & 87.60 & 8772 & 92.01 & 6525 & 94.17\\
      \midrule
      \multirow{6}{*}{Russian} & \multirow{3}{*}{\shortstack[l]{mBERT\\uncased}} & 3 & 2655 & 27.12 & 2835 & 49.73 & 1102 & 62.47 & 880 & 72.83 & 843 & 79.04\\
       &  & 2 & 5173 & 31.76 & 4262 & 55.84 & 1787 & 64.95 & 1361 & 74.80 & 1268 & 80.24\\
       &  & 1 & 23530 & 42.86 & 12633 & 65.49 & 8414 & 70.22 & 6244 & 79.37 & 5281 & 82.98\\
       & \multirow{3}{*}{\shortstack[l]{mBERT\\cased}} & 3 & 1143 & 40.87 & 1184 & 67.32 & 1006 & 66.96 & 784 & 77.29 & 807 & 79.91\\
       &  & 2 & 2483 & 45.04 & 2033 & 70.81 & 1558 & 68.93 & 1226 & 78.78 & 1229 & 81.20\\
       &  & 1 & 14929 & 55.07 & 8308 & 76.36 & 7447 & 72.81 & 5767 & 81.93 & 5169 & 83.83\\
    \bottomrule
  \end{tabular}
\end{table*}
